# Supplementary material for: Superionic Ionic Conductor Discovery via Multiscale Topological Learning
Source: arXiv:2412.11398 source file (2024-12-16)
Supplement: Supplementary file 1 [file SupplementaryInformation.pdf]

*Supplementary Information*

# Superionic Ionic Conductor Discovery via Multiscale Topological Learning


Dong Chen[*1,2], Bingxu Wang[†1], Shunning Li[1], Wentao Zhang[1], Kai Yang[1], Yongli Song[1], Guo-Wei Wei [‡2,4] and Feng Pan [§1]

[1]School of Advanced Materials, Peking University, Shenzhen Graduate School, Shenzhen 518055, China

[2]Department of Mathematics, Michigan State University, MI, 48824, USA

[3]Department of Electircal and Computer Engineering, Michigan State University, MI 48824, USA

[4]Department of Biochemistry and Molecular Biology, Michigan State University, MI 48824, USA

[*]contributed equally to this work

[†]contributed equally to this work

[‡]Corresponding author: weig@msu.edu

[§]Corresponding author: panfeng@pkusz.edu.cn

Table S1. The number of compounds that passed each steps of the high-throughput screening of crystal structural framework.

| **Screening Step** | **Number of Compositions** |
|---|---|
| Remove Duplicate | 2590 |
| Filter Connection Radius | 1443 |
| Filter Servive Betti1 | 770 |
| Clustering Methods | 339 |
| Final screening | 43 |

Table S2. List of known LSICs

| **ICSD-IDs** | **Compositions** | **Superionic conductor** |
|---|---|---|
| 100169 | $Li_{14}Zn(GeO_4)_4$ | LISCISON |
| 157654 | $Li_7P_3S_{11}$ | $Li_7P_3S_{11}$ |
| 163297 | $Li_{1.2}(Al_{0.2}Ge_{0.2}Ti_{1.6})$ $(PO_4)_3$ | NASICON |
| 188887 | $Li_{10}GeP_2S_{12}$ | LGPS |
| 422259 | $Li_7La_3Zr_2O_{12}$ | LLZO |
| 50422 | $Li_{2.64}(Sc_{0.9}Ti_{0.1})_2(PO_4)_3$ | $Li_3A_2(PO_4)_3$ |
| 35018 | $Li_3PS_4$ | Li-P-S |
| 92200 | $Li_4GeS_4$ | Li-Ge-S |
| 174202 | $Li_7La_3Hf_2O_{12}$ | Garnet |
| 191542 | $Li_{6.46}Al_{0.08}1La_3Zr_2O_{12}$ | Garnet |
| 185539 | $Li_{6.06}Al_{0.20}1La_3Zr_2O_{12}$ | Garnet |
| 185540 | $Li_{6.06}Al_{0.20}1La_3Zr_2O_{12}$ | Garnet |
| 238693 | $La_3Li_{5.8}Zn_{0.6}Zr_2O_{12}$ | Garnet |
| 238692 | $La_3Li_{5.8}Zn_{0.6}Zr_2O_{12}$ | Garnet |
| 238690 | $Al_{0.24}La_3Li_{6.28}Zr_2O_{12}$ | Garnet |
| 238689 | $Al_{0.24}La_3Li_{6.28}Zr_2O_{12}$ | Garnet |
| 195182 | $(Li_{6.26}Al_{0.24})La_3Zr_2O_{12}$ | Garnet |
| 69076 | $La_3Li_5Sb_2O_{12}$ | Garnet |
| 174612 | $Li_6(CaLa_2)Sb_2O_{12}$ | Garnet |
| 174615 | $Li_{6.4}(Ca_{1.4}La_{1.6})Sb_2O_{12}$ | Garnet |
| 174617 | $Li_{6.4}(Ca_{1.4}La_{1.6})Sb_2O_{12}$ | Garnet |
| 158373 | $Li_6SrLa_2Bi_2O_{12}$ | |
| 161342 | $Li_5La_3(Sb_2O_{12})$ | Garnet |
| 161343 | $Li_5La_3(Sb_2O_{12})$ | Garnet |
| 161389 | $Li_5La_3(SbO_6)_2$ | Garnet |
| 163914 | $Li_7La_3Sn_2O_{12}$ | Garnet |
| 182034 | $Li_7La_3Sn_2O_{12}$ | Garnet |
| 182035 | $Li_{2.25}H_{4.75}La_3Sn_2O_{12}$ | Garnet |
| 182036 | $Li_{4.59}H_{2.41}La_3Sn_2O_{12}$ | Garnet |
| 245641 | $Li_5La_3(SbO_6)_2$ | Garnet |

| | | |
|---|---|---|
| 245934 | $Li_6SrLa_2Sb_2O_{12}$ | Garnet |
| 245935 | $Li_{6.4}Sr_{1.4}La_{1.6}Sb_2O_{12}$ | Garnet |
| 246817 | $Li_7La_3Zr_2O_{12}$, | Garnet |
| 261302 | $Li_7La_3Zr_2O_{12}$, | Garnet |
| 183684 | $Li_7La_3Zr_2O_{12}$, | LLZO |
| 183685 | $Li_7La_3Zr_2O_{12}$, | Garnet |
| 184230 | $Li_7La_3(ZrO_6)_2$ | Garnet |
| 191528 | $Li_7La_3Zr_2O_{12}$, | Garnet |
| 183607 | $Li_7La_3Zr_2O_{12}$, | Garnet |
| 238687 | $Li_7La_3Zr_2O_{12}$, | Garnet |
| 238686 | $Li_7La_3Zr_2O_{12}$, | Garnet |
| 65025 | $Li_2Mg_2(SO_4)_3$ | $Li_3A_2(PO_4)_3$ |
| 62300 | $Li_3Sc_2(PO_4)_3$ | $Li_3A_2(PO_4)_3$ |
| 91113 | $Li_{2.72}Ti_2(PO_4)_3$ | $Li_3A_2(PO_4)_3$ |
| 202539 | $Li_{2.68}(Ti_{1.86}Al_{0.14})(PO_4)_3$, | NASICON |
| 94029 | $(Li_{0.72}Na_{0.88})(Ti_{1.4}Al_{0.6})(PO_4)_3$ | NASICON |
| 94030 | $(Li_{1.09}Na_{0.71})(Ti_{1.2}Al_{0.8})(PO_4)_3$ | NASICON |
| 94031 | $(Li_{1.45}Na_{0.45})(Ti_{1.1}Al_{0.9})(PO_4)_3$ | NASICON |
| 163299 | $Li_{1.2}(Al_{0.2}Ge_{0.4}Ti_{1.4})(PO_4)_3$ | NASICON |
| 163300 | $Li_{1.4}(Al_{0.4}Ge_{0.4}Ti_{1.2})(PO_4)_3$ | NASICON |
| 163301 | $Li_{1.6}(Al_{0.6}Ge_{0.4}Ti)(PO_4)_3$ | NASICON |
| 163302 | $Li_{1.2}(Al_{0.2}Ge_{0.6}Ti_{1.2})(PO_4)_3$ | NASICON |
| 163303 | $Li_{1.4}(Al_{0.4}Ge_{0.6}Ti)(PO_4)_3$ | NASICON |
| 163304 | $Li_{1.6}(Al_{0.6}Ge_{0.6}Ti_{0.8})(PO_4)_3$ | NASICON |
| 163305 | $Li_3Ti_2(PO_4)_3$, $Li_{2.93}Ti_2(PO_4)_3$ | NASICON |
| 193036 | $Li_{2.93}Ti_2(PO_4)_3$ | NASICON |
| 193037 | $Li_{2.8}Ti_2(PO_4)_3$, | NASICON |
| 193032 | $Li_{1.2}(Al_{0.2}Ge_{0.6}Ti_{1.2})(PO_4)_3$ | NASICON |
| 193038 | $Li_3Ti_2(PO_4)_3$ | NASICON |
| 193033 | $Li_{1.6}(Al_{0.6}Ge_{0.4}Ti)(PO_4)_3$ | NASICON |
| 92250 | $LiZr_2(PO_4)_3$ | $Li_3A_2(PO_4)_3$ |
| 97658 | $Li_2Ti_2(PO_4)_3$ | NASICON |
| 97659 | $Li_{2.96}(Sc_{0.9}Zr_{0.1})_2(PO_4)_3$ | NASICON |
| 97660 | $LiZr_2(PO_4)_3$ | NASICON |
| 191891 | $Li_{1.15}(Y_{0.15}Zr_{1.85})(PO_4)_3$ | NASICON |
| 245527 | $Li_{0.7}La_{0.1}Zr_2(PO_4)_3$ | NASICON |
| 257190 | $Li_{1.12}Ti_{1.88}In_{0.12}(PO_4)_3$ | NASICON |
| 20208 | $Li_3(PO_4)$ | LISICON |
| 25816 | $Li_3Zn_{0.5}(GeO_4)$ | LISICON |
| 34221 | $Li_{2.5}Ga_{0.5}GeO_4$ | LISICON |
| 50058 | Li3PO4 | Li-P-O |
| 79427 | $Li_{3.5}Zn_{.25}GeO_4$ | LISICON |
| 77095 | $Li_{14}Zn(GeO_4)_4$ | LISICON |

| | | |
|---|---|---|
| 8280 | $Li_2MgGeO_4$ | LISICON |
| 65643 | $Li_{2.5}Ga_{0.5}GeO_4$ | LISICON |
| 78513 | $Li_3Zn_{.5}GeO_4$ | LISICON |
| 100167 | $Li_{3.5}Zn_{.25}GeO_4$ | LISICON |
| 100169 | $Li_{6.6}SiPO_8$ | LISICON |
| 202631 | $Li_3PO_4$ | LISICON |
| 202632 | $Li_{2.5}Ga_{0.5}GeO_4$ | LISICON |
| 166547 | $Li_2MgGeO_4$ | LISICON |
| 238601 | $Li_{2.5}Ga_{0.5}GeO_4$ | LISICON |
| 290831 | $Li_4SnS_4$ | Li-Ge-S |
| 290832 | $Li_4SnS_4$ | Li-Ge-S |
| 50578 | $Li_4GeS_4$ | Li-Ge-S |
| 92200 | $Li_4GeS_4$ | Li-Ge-S |
| 95649 | $Li_4GeS_4$ | Li-Ge-S |
| 188886 | $Li_{10}(GeP_2S_{12})$ | LGPS |
| 188887 | $Li_{10}(SnP_2S_{12})$ | LGPS |
| 193755 | $Li_{10.35}((Ge_{1.35}P_{1.65})S_{12})$ | LGPS |
| 193947 | $Li_{10.35}Si_{1.35}P_{1.65}S_{12}$ | LGPS |
| 241439 | $Li_{9.81}Sn_{0.81}P_{2.19}S_{12}$ | LGPS |
| 252036 | $Li_{10}(Ge_{0.416}Sn_{0.584})P_2S_{12}$ | LGPS |
| 252037 | $Li_{10}(Ge_{0.776}Sn_{0.224})P_2S_{12}$ | LGPS |
| 252038 | $Li_{10.35}(Sn_{0.27}Si_{1.08})$, $P_{1.65}S_{12}$ | LGPS |
| 252039 | $Li_{10.35}(Sn_{0.27}Si_{1.08})$, $P_{1.65}S_{12}$ | LGPS |
| 252040 | $Li_{10.5}(Sn_{0.2}Si_{0.8})_{1.5}P_{1.5}S_{12}$ | LGPS |
| 252041 | $Li_{10.2}(Sn_{0.2}Si_{0.8})_{1.2}P_{1.8}S_{12}$ | LGPS |

Table S3. Oxide compounds that passed the high-throughput screening of crystal structural framework but rejected by other considerations.

| **ICSD-IDs** | **Compositions** | **Reasons** |
|---|---|---|
| 19024, 27007, 27008, 30964, 33809, 33810, 36532, 56443, 60363, 61086, 61087, 65127, 78059, 84240, 96224, 239794, 243972, 253007, 257739, 281011, 415121, 416926, 416927, 416928, 416929, 417653, 421259, 421549, 423635, 432026, 19023, 67238, 92571, 421548, 260280 | $Li_2CaGeO_4$, $Na_3Li_3Sc_2F_{12}$, $Na_3Li_3In_2F_{12}$, KLiO, $Cs_2Li_2(SiO_4)$, $Cs_2Li_2(TiO_4)$, $Cs_2Li_2(GeO_4)$, LiSrP, $Na_3Li_3Ti_2F_{12}$, $Rb_2Li_2SiO_4$, $Rb_2Li_2GeO_4$, $LiGaGeO_4$, $Li_2(TiSiO_5)$, $Li(Al_7B_4O_{17})$, $LiSr(GaN_2)$, $LiSc(SeO_3)_2$, $LiCsCO_3$, $LiGaGe_2Se_6$, $LiGaGeO_4$, $Li_2PbGeS_4$, $Li_2(TeSe_3)$, $Li_3Na_3(InF_6)_2$, $Li_6Y_3(PS_4)_5$, $Li_4Sr_3(Si_2N_6)$, $SrLi_2N_4Si_2$, $CsLi_2Cl_3$, | Bad Li network |

| | | |
|---|---|---|
| | $Li_3Y(BO_3)_2$, $Li_2CaSiO_4$, $LiAlGeO_4$, $KLi(CO_3)$, $CaLi_2N_4Si_2$, $Li_2Zn_3(P_2O_7)_2$ | |
| 610785 | $Li_3As$ | Binary compounds |
| 90147 | $Cs_{14}Li_{22.72}(Li_{18.4}Si_{72}O_{172})(D_2O)_{6.16}$ | Containing $D_2O$ |
| 88334 | $Li_6(P_6O_{18})(H_2O)_{9.86}$ | Containing H |
| 6269, 67925, 171366, 62586, 428547 | $Li_{0.91}(Al_{0.91}Si_{1.09}O_4)(H_2O)_{0.98}$, $Li_8(HPO_4)(Be_6P_6O_{24})(H_2O)$, $K_{2.6}Li_{5.4}(Li_4Si_{16}O_{38})(H_2O)_{4.3}$, $Li_4(P_4O_{12})(H_2O)_5$, $(Li_2(H_2O)_7)Se$ | Containing $H_2O$ |
| 251594 | $Li_6RbB_2O_6F$ | Containing O and F |
| 50992 | $Li(Y_{0.95}Eu_{0.05})O_2$ | Containing Y, Eu |
| 432591 | $Li_4PN_3$ | High-pressure hynthesis. The product is sensitive to traces of air and moisture. |
| 161763, 250297, 50612 | $Li_2Ga_2GeS_6$, $Li_2Ti(GeO_4)O$, $Li_3Sc_2(PO_4)_3$, $Li_2(BAlO_4)$ | ehull>50emV |
| 188886, 188887, 193755, 193947, 241439, 252036, 252037, 252038, 252039, 252040, 252041, 255747, 255748, 255749, 257946, 257947, 257948 | $Li_{10}(GeP_2S_{12})$, $Li_{10}(SnP_2S_{12})$, $Li_{10.35}((Ge_{1.35}P_{1.65})S_{12})$, $Li_{10.35}Si_{1.35}P_{1.65}S_{12}$, $Li_{9.81}Sn_{0.81}P_{2.19}S_{12}$, $Li_{10}(Ge_{0.416}Sn_{0.584})P_2S_{12}$, $Li_{10}(Ge_{0.776}Sn_{0.224})P_2S_{12}$, $Li_{10.35}(Sn_{0.27}Si_{1.08})$, $P_{1.65}S_{12}$, $Li_{10.5}(Sn_{0.2}Si_{0.8})_{1.5}P_{1.5}S_{12}$, $Li_{10.2}(Sn_{0.2}Si_{0.8})_{1.2}P_{1.8}S_{12}$ | LGPS |
| 161342, 161343, 161389, 163914, 174202, 174612, 174613, 174614, 174615, 174616, 174617, 182034, 182035, 182036, 183607, 183685, 184230, 185539, 185540, 191528, 191542, 195182, 238686, 238687, 238689, 238690, 238692, 238693, 241475, 245641, 245934, 245935, 246817, 253056, 261302, 430571, 430575, 430576, 430602, 69076 | $Li_5La_3(Sb_2O_{12})$, $Li_6(SrLa_2)(Sb_2O_{12})$, $Li_5La_3(SbO_6)_2$, $Li_7La_3Sn_2O_{12}$, $Li_7La_3Hf_2O_{12}$, $Li_6(CaLa_2)Sb_2O_{12}$, $Li_{6.4}(Ca_{1.4}La_{1.6})Sb_2O_{12}$, $Li_7La_3Sn_2O_{12}$, $Li_{2.25}H_{4.75}La_3Sn_2O_{12}$, $Li_{4.59}H_{2.41}La_3Sn_2O_{12}$, $Li_7La_3Zr_2O_{12}$, $Li_7La_3(ZrO_6)_2$, $Li_{6.06}Al_{0.20}La_3Zr_2O_{12}$, $Li_7La_3Zr_2O_{12}$, $Li_{6.46}Al_{0.081}La_3Zr_2O_{12}$, $(Li_{6.26}Al_{0.24})La_3Zr_2O_{12}$, $La_3Li_7Zr_2O_{12}$, $Al_{0.24}La_3Li_{6.28}Zr_2O_{12}$, $La_3Li_{5.8}Zn_{0.6}Zr_2O_{12}$, $Li_{51.2}Al_{1.6}La_{24}Zr_{16}O_{96}$, $Li_5La_3(SbO_6)_2$, $Li_5La_3(SbO_6)_2$, | Garnet |

| | | |
|---|---|---|
| | $Li_{6.4}Sr_{1.4}La_{1.6}Sb_2O_{12}$, $Li_7La_3Zr_2O_{12}$, $Li_7La_3Hf_2O_{12}$, $Li_{5.91}Al_{0.216}La_{2.95}Zr_2O_{12}$, $Al_{0.11}Ga_{0.08}La_{2.94}Li_{6.85}Zr_2O_{12}$, $Al_{0.19}Ga_{0.05}La_{2.88}Li_{5.55}O_{12}Zr_2$, $Li_{6.55}Ga_{0.05}La_{2.91}Zr_2O_{12}$, $La_3Li_5Sb_2O_{12}$ | |
| 23017, 38350, 50421, 68494, 253896, 431368, 431573, 642303, 35405, 65445, 255464, 40247, 55665, 72100, 35290, 65126, 73223, 79098, 8372, 169799, 26817, 249872, 249873, 254974 | $Li_4Zn(PO_4)_2$, $Li_4PbO_4$, $Li_{3.2}Sc_2(PO_4)_3$, $Li_{10}(Zn_4O_9)$, $Li_{10}Si_2P_6$, $Li_2SiP_2$, $LiSbS_2$, $Rb_2Li_{14}(Pb_3O_{14})$, $K_2Li_{14}(Zr_3O_{14})$, $Li_4Zn(PO_4)_2$, $Li_6TeO_6$, $LiAlSiO_4$, $Li_3GaSiO_5$, $LiAlSi_2O_6$, $Li_3AsS_3$, $K_2Li_3GaO_4$, $LiAlGeO_4$, $Li_2ZnBr_4$, $Li_5La_3Bi_2O_{12}$, $Li_{2.2}Zn_{0.8}P_2O_7$ , $Li_2CdGeS_4$, $Li_2CdSnS_4$, $Li_2CdGeSe_4$ | Duplicate structure |
| 47143, 47144, 47145, 428002, 14364, 67702, 67703, 95407, 239962, 254107, 30276 | $Li_{3.175}(SiO_4)_{0.7}(SO_4)_{0.3}$, $Li_{3.17}Si_{0.7}S_{0.3}O_4$, $Li_{3.4}Si_{0.7}S_{0.3}O_4$, $Li_5(B(SO_4)_4)$, $LiNa(SO_4)$, $Li_4(SO_4)_2$, $LiNaSO_4$, $Li_2SO_4$ | Containing $SO_4^{2-}$ |
| 25308, 42062, 42068, 171497, 419577, 426692, 429881 | $Li_9Ge_4$, LiGe, $Li_{11}Ge_6$, $Li_8Zn_2Ge_3$, $Ge_{12}Li_7$, $Li_{18}Na_2Ge_{17}$, $Li_3NaGe_2$ | Germanide, Ge unusual valence state |
| 26298, 80593, 255465, 255466, 255468, 264522, 78514, 153218, 255467 | $(Sr_7Li_4Si_{10})_{0.1429}$, $Li_{2.5}Al_{0.5}(SiO_4)$, $Li_4Zn(PO_4)_2$, $Li_{3.7}Zn_{0.7}Ga_{0.3}(PO_4)_2$, $Li_{3.5}Zn_{0.5}Ga_{0.5}(PO_4)_2$, $Hf_2La_3(Li_{6.74}Al_{0.08})O_{12}$, $Li_{2.42}Ga_{0.58}GeO_4$, $Li_{2.46}Al_{0.18}(BO_3)$, $Li_{3.7}Zn_{0.7}Ga_{0.3}(PO_4)_2$ | Li sharing sites with: Si, Al, Zn, Ga |
| 50422, 62300, 65025, 71277, 91113, 92250 | $Li_{2.64}(Sc_{0.9}Ti_{0.1})_2(PO_4)_3$, $Li_3Sc_2(PO_4)_3$, $Li_2Mg_2(SO_4)_3$, $Li_{2.72}Ti_2(PO_4)_3$, $LiZr_2(PO_4)_3$ | $Li_3A_2(PO_4)_3$ |
| 1037, 16229 | $Li_5AlO_4$ | Li-Al-O |
| 433369 | $Li_5AlS_4$ | Li-Al-S |
| 165579, 413238 | $Li(ClO_4)$ | Li-Cl-O |
| 31050, 100403 | $Li_6Ge_2O_7$, $Li_2(GeO_3)$ | Li-Ge-O |
| 50578, 92200, 95649, 290831, 290832 | $Li_4GeS_4$, $Li_4SnS_4$ | Li-Ge-S |
| 638, 50058, 79426, 85714, 246859, 248414, 257439 | LiPO3, Li3PO4, $Li2_{.88}PO_{3.73}N_{0.14}$, $Li_6P_6O_{18}$, $Li_4P_2O_7$ | Li-P-O |
| 35018, 157654, 180318, | $Li_3PS_4$, $Li_7(P_3S_{11})$, $Li_4P_2S_6$ | Li-P-S |

| | | |
|---|---|---|
| 242170 | | |
| 48106 | $Li_2SeO_4$ | Li-Se-O |
| 8280, 20031, 20208, 25816, 34221, 65643, 77095, 78513, 79427, 100167, 100169, 166547, 202631, 202632, 238601, 257440 | $Li_2MgGeO_4$, $Li_2CdGeO_4$, $Li_3(PO_4)$, $Li_3Zn_{0.5}(GeO_4)$, $Li_{2.5}Ga_{0.5}GeO_4$, $Li_{14}Zn(GeO_4)_4$, $Li_2Mg(GeO_4)$, $Li_3Zn_{.5}GeO_4$, $Li_{3.5}Zn_{.25}GeO_4$, $Li_{6.6}SiPO_8$, $Li_3PO_4$ | LISICON |
| 65176 | $Li_8O_2SiO_4$ | Li-Si-O |
| 58, 2512, 23723, 59243, 153806, 431359 | $Li_2SO_4$, $Li_4P_2O_7$, $Li_2S_5O_{16}$ | Li-S-O |
| 415120 | $Li_2TeS_3$ | Li-Te-S |
| 16219 | $Li_5TlO_4$ | Li-Tl-O |
| 75164 | $Li_4TiO_4$ | Li-Ti-O |
| 59646, 59647, 99395, 99396, 99397, 99398, 99399, 99402, 236888 | $(La_{0.62}Li_{0.16})(TiO_3)$, $(Li_{0.18}La_{0.122})La_{0.483}(TiO_3)$, $(Li_{0.18}La_{0.119})La_{0.483}(TiO_3)$, $(Li_{0.18}La_{0.118})La_{0.484}(TiO_3)$, $(Li_{0.18}La_{0.123})La_{0.485}(TiO_3)$, $(Li_{0.18}La_{0.118})La_{0.492}(TiO_3)$, $(Li_{0.18}La_{0.121})La_{0.482}(TiO_3)$, $La_{4.44}Li_{2.66}Ti_8O_{24}$ | LLTO |
| 183684, 238685, 238688, 238691, 422259, 83652 | $Li_7La_3Zr_2O_{12}$, $La_3Li_7Zr_2O_{12}$, $Al_{0.24}La_3Li_{6.28}Zr_2O_{12}$, $La_3Li_{5.8}Zn_{0.6}Zr_2O_{12}$, $Li_7La_3Zr_2O_{12}$ | LLZO |
| 254406 | $LiGaGe_2S_6$ | Low Melting Point |
| 1384, 243929, 264211, 391200, 421083, 426103 | $Li(SO_3F)$, $Li_{24}Sr_{12}(Si_{24}N_{47}O)F$, $Li_{40.70}Y_{3.30}Ca_{5.70}(Li_2Si_{30}N_{59})O_2F$, $Li_{5.88}H_{4.5}(P_{12}O_2N_{22})Cl_{2.556}$, $Li_6(PS_4)(SI)$, $Li_9Mg_3(PO_4)_4F_3$ | Multiple anions |
| 63018, 94029, 94030, 94031, 95980, 95981, 163297, 163298, 163299, 163300, 163301, 163302, 163303, 163304, 163305, 193032, 193033, 193034, 193035, 193036, 193037, 193038, 193039, 193040, 193041, 202538, 202539, 257190, 261825, 50423, 97658, 97659, 97660, 191891, 245527 | $Li_{1.15}Ti_{1.85}In_{0.15}P_3O_{12}$, $(Li_{0.72}Na_{0.88})(Ti_{1.4}Al_{0.6})(PO_4)_3$, $(Li_{1.09}Na_{0.71})(Ti_{1.2}Al_{0.8})(PO_4)_3$, $(Li_{1.45}Na_{0.45})(Ti_{1.1}Al_{0.9})(PO_4)_3$, $Li_{3.18}Ti_2(PO_4)_3$, $Li_{1.2}(Al_{0.2}Ge_{0.2}Ti_{1.6})(PO_4)_3$, $Li_{1.4}(Al_{0.4}Ge_{0.2}Ti_{1.4})(PO_4)_3$, $Li_{1.6}(Al_{0.6}Ge_{0.2}Ti_{1.2})(PO_4)_3$, $Li_{1.2}(Al_{0.2}Ge_{0.4}Ti_{1.4})(PO_4)_3$, $Li_{1.4}(Al_{0.4}Ge_{0.4}Ti_{1.2})(PO_4)_3$, $Li_{1.6}(Al_{0.6}Ge_{0.4}Ti)(PO_4)_3$, $Li_{1.2}(Al_{0.2}Ge_{0.6}Ti_{1.2})(PO_4)_3$, $Li_{1.4}(Al_{0.4}Ge_{0.6}Ti)(PO_4)_3$, $Li_{1.6}(Al_{0.6}Ge_{0.6}Ti_{0.8})(PO_4)_3$, | NASICON |

| | | |
|---|---|---|
| | $Li_3Ti_2(PO_4)_3$, $Li_{2.93}Ti_2(PO_4)_3$, $Li_{2.8}Ti_2(PO_4)_3$, $Li_3(Ti_{1.82}Al_{0.18})(PO_4)_3$, $Li_3(Ti_{1.79}Al_{0.21})(PO_4)_3$, $Li_3(Ti_{1.78}Al_{0.22})(PO_4)_3$, $Li_3(Ti_{1.83}Al_{0.17})(PO_4)_3$, $Li_{2.8}(Ti_{1.82}Al_{0.18})(PO_4)_3$, $Li_{2.68}(Ti_{1.86}Al_{0.14})(PO_4)_3$, $Li_{1.12}Ti_{1.88}In_{0.12}(PO_4)_3$, $Li_{1.15}Ti_{1.85}In_{.15}(PO_4)_3$, $Li_{1.3}Al_{0.3}Ti_{1.7}(PO_4)_3$, $Li_2Ti_2(PO_4)_3$, $Li_{2.96}(Sc_{0.9}Zr_{0.1})_2(PO_4)_3$, $LiZr_2(PO_4)_3$, $Li_{1.15}(Y_{0.15}Zr_{1.85})(PO_4)_3$, $Li_{0.7}La_{0.1}Zr_2(PO_4)_3$ | |
| 432318 | $Li_{141}N_{126}B_9P_{42}$ | Number atoms > 500, further calculations due |
| 60774, 100465, 642222 | Li3P7, LiP | P unusual valence state |
| 78836, 107304 | $Li_5NBr_2$, LiCaN | Redox reactions without the participation of Li |
| 100020 | $Li_2Sb$ | Sb unusual valence state |
| 67359, 193768, 264695 | LiNaSe, $Li_4SnSe_4$, $Li_2ZnSe_2O_6$ | Selenide |
| 431316 | $Li_{18}N_{16}P_6$ | sigma,348k,7.7E-8 to 1.46E-6; E_a=48.3kJ/mol |
| 24146, 41023, 87408, 281277, 430497, 642372 | $Li_2Si$, $Li_8MgSi_6$, $Li_{2.35}Si$, $Al_{3.39}Li_{14.61}Si_6$, $Li_{11.56}Na_{0.44}Si_7$ | Silicide |
| 182961 | $(Li_2(Ti_3O_7))_{1.143}$ | Ternary oxides containing Ti |
| 250066 | $Li_{3.05}Ge_{0.31}P_{0.69}O_4$ | Excluded from further calculations due to the large number of fractional occupied ions in the unit cell |
| 26472, 409657 | LiAs, $As_7Li_3$ | As unusual valence state |
| 158373, 238600, 255750, 420126 | $Li_6SrLa_2Bi_2O_{12}$, $Li_{6.5}Si_{0.5}P_{1.5}O_8$, $Li_{10}SnP_2S_{12}$, $Li_2SiN_2$ | Very high conductive after doped |

Table S4. Oxide compounds that passed the high-throughput screening of crystal structural framework

| **ICSD-IDs** | **Compositions** | **Structure Type** |
|---|---|---|
| 1411 | $Li_4(PbO_4)$ | $Li_4PbO_4$ |
| 2319 | $Li_2BeSiO_4$ | $Li_2BeSiO_4(oS_{32})$ |
| 4317 | $Li_2TeO_3$ | $Li_2TeO_3$ |
| 6169 | $Li_6Al_2(BO_3)_4$ | $Li_3AlB_2O_6$ |
| 8237 | $Li_2Zn(SiO_4)$ | $Li_2ZnSiO_4$ |

| | | |
|---|---|---|
| 9987 | $Li_6Ga_2(BO_3)_4$ | $Li_3AlB_2O_6$ |
| 15631 | $Li_7(SbO_6)$ | |
| 23634 | $Li_{10}(Zn_4O_9)$ | |
| 26297 | $Li_6(TeO_6)$ | $Li_6TeO_6$ |
| 26817 | $LiAl(Si_2O_6)$ | $LiAlSi_2O_6$ |
| 35250 | $K_2Li_{14}(Pb_3O_{14})$ | $K_2Li_{14}Pb_3O_4$ |
| 37071 | $Li_3Na_2(GaO_4)$ | $Li_3Na_2GaO_4$ |
| 38324 | $Li_3KGeO_4$ | $CsNa_3TiO_4$ |
| 40245 | $Li_3BiO_3$ | |
| 40457 | $LiSbS_2$ | $AgAsS_2$ |
| 50950 | $LiZn(PO_4)$ | $LiZnPO_4$ |
| 59381 | $Li_3(AsS_3)$ | |
| 59640 | $Li_4Zn(PO_4)_2$ | $Li_4O_8P_2Zn$ |
| 61204 | $Na_4Li_5(BO_3)_3$ | |
| 67991 | $Li_{14}Be_5B(BO_3)_9$ | |
| 69967 | $NaLi_2(PO_4)$ | $Li_3PO_4$ |
| 71035 | $KLi_6(BiO_6)$ | $KLi_6IrO_6$ |
| 72840 | $Li_6K(BiO_6)$ | |
| 74864 | $CsKNa_2Li_8(Li(SiO_4))_4$ | $CsKNa_2Li_8(LiSiO_4)_4$ |
| 74865 | $RbNa_3Li_8(Li(SiO_4))_4$ | $CsKNa_2Li_8(LiSiO_4)_4$ |
| 78326 | $Li_{10}(Si_2PbO_{10})$ | |
| 78819 | $Li_{10}N_3Br$ | |
| 86184 | $LiZn(AsO_4)$ | $LiGaSiO_4$ |
| 86458 | $Li_3Sc_2(PO_4)_3$ | $Li_3Fe_2(PO_4)_3$ |
| 87596 | $Li_2(TiO)(SiO_4)$ | $Li_2TiSiO_5$ |
| 92708 | $Li(AlSiO_4)$ | $LiGaSiO_4$ |
| 95972 | $Li_2(MgSiO_4)$ | $Li_2ZnSiO_4$ |
| 202115 | $NaLi_3(SiO_4)$ | $NaLi_3SiO_4$ |
| 202116 | $NaLi_3GeO_4$ | $NaLi_3SiO_4$ |
| 241234 | $Li_3Sc(BO_3)_2$ | |
| 252215 | $Li_3AlSiO_5$ | $AlFeO_3$ |
| 253895 | $Li_{10}Si_2P_6$ | |
| 257740 | $LiGa_{0.5}Al_{0.5}GeO_4$ | $LiGaSiO_4$ |
| 262642 | $In_2Li_2SiS_6$ | $Cd_4GeS_6$ |
| 262643 | $In_2Li_2GeS_6$ | $Cd_4GeS_6$ |
| 402341 | LiBeN | |
| 413355 | $(LiI)_2(Li_3(SbS_3))$ | |
| 424834 | $Li_3SbS_3$ | |
| 424835 | $Li_3AsS_3$ | |
| 431367 | $Li_2SiP_2$ | |

Table S5. Ionic conductivity at 800 K, 1000 K, 1200 K, and 1400 K and room temperature (300K) and activation barrier of oxide compounds that passed the high-throughput screening of crystal structural framework

| ICSD-IDs | Compositions | Ionic conductivity | | | | | Activation barrier |
|---|---|---|---|---|---|---|---|
| | | 800K | 1000K | 1200K | 1400K | 300K | |
| 1411 | $Li_4(PbO_4)$ | 1.146 | 5.196e-1 | 4.740e+1 | 3.473e+3 | 4.341e-15 | 1.345 |
| 2319 | $Li_2BeSiO_4$ | 7.644e-1 | 5.898e-1 | 1.579e-1 | 2.377e-1 | 7.724e+1 | -0.148 |
| 4317 | $Li_2TeO_3$ | 1.782 | 6.974e-10 | 1.542e+2 | 8.987e+2 | 6.879e-22 | 1.729 |
| 6169 | $Li_6Al_2(BO_3)_4$ | 2.396e+1 | 1.490e+1 | 3.967e+1 | 5.567e-10 | 3.515e+34 | -2.935 |
| 8237 | $Li_2Zn(SiO_4)$ | 2.739e-1 | 7.158e-10 | 8.013e-2 | 5.113e-10 | 1.708e+19 | -1.973 |
| 9987 | $Li_6Ga_2(BO_3)_4$ | 1.266 | 4.612e+1 | 1.698e+2 | 8.764e+1 | 1.291e-8 | 0.826 |
| 15631 | $Li_7(SbO_6)$ | 7.079e+2 | 1.119e+3 | 1.491e+3 | 1.642e+3 | 7.634e | 0.228 |
| 23634 | $Li_{10}(Zn_4O_9)$ | 5.251 | 3.960e+1 | 9.849e+1 | 1.359e+2 | 4.694e-6 | 0.624 |
| 26297 | $Li_6(TeO_6)$ | 2.822 | 8.745e-1 | 5.879e-1 | 9.491e-10 | 7.908e+30 | -2.71 |
| 26817 | $LiAl(Si_2O_6)$ | 8.973e+1 | 1.302e+2 | 2.644e+2 | 2.456e+2 | 3.194e-1 | 0.272 |
| 35250 | $K_2Li_{14}(Pb_3O_{14})$ | 1.122 | 5.584e-1 | 4.608e+1 | 2.170e+2 | 3.291e-11 | 0.998 |
| 37071 | $Li_3Na_2(GaO_4)$ | 5.986e-1 | 2.907e-1 | 1.648e-1 | 6.053e-10 | 5.059e+28 | -2.567 |
| 38324 | $Li_3KGeO_4$ | 2.183 | 8.618e-10 | 7.182e-10 | 7.627e+2 | 1.359e-4 | 0.056 |
| 40245 | $Li_3BiO_3$ | 6.923e+1 | 7.249e+2 | 7.665e+2 | 1.669e+3 | 2.327e-4 | 0.573 |
| 40457 | $LiSbS_2$ | 5.444e+1 | 2.734e+1 | 1.143e+2 | 2.578e+2 | 1.897e-2 | 0.349 |
| 50950 | $LiZn(PO_4)$ | 6.880e-1 | 8.750e-1 | 1.108e-1 | 2.157e-1 | 1.600e+2 | -0.176 |
| 59381 | $Li_3(AsS_3)$ | 1.056e+3 | 1.975e+3 | 2.058e+3 | 3.407e+3 | 5.220 | 0.260 |
| 59640 | $Li_4Zn(PO_4)_2$ | 1.220e+2 | 4.183e+1 | 1.568e+2 | 9.221e+2 | 1.320e-2 | 0.387 |
| 61204 | $Na_4Li_5(BO_3)_3$ | 4.649e-1 | 7.186e-10 | 3.186e+1 | 2.645e+2 | 6.732e-22 | 1.693 |
| 67991 | $Li_{14}Be_5B(BO_3)_9$ | 9.244e-1 | 5.546e-1 | 7.154e-10 | 1.144e+2 | 6.494e+5 | -0.591 |
| 69967 | $NaLi_2(PO_4)$ | 9.218e-1 | 1.588e-2 | 2.441 | 3.572 | 1.516e-5 | 0.429 |
| 71035 | $KLi_6(BiO_6)$ | 2.294e+1 | 2.622e+1 | 1.322e+1 | 1.336e+2 | 6.162e-2 | 0.272 |
| 72840 | $Li_6K(BiO_6)$ | 1.329 | 8.498e-1 | 5.465e-1 | 1.205e+2 | 4.792e-7 | 0.611 |
| 74864 | $CsKNa_2Li_8(Li(SiO_4))_4$ | 2.780e-1 | 1.509e+1 | 3.397 | 1.002 | 1.885e-3 | 0.297 |
| 74865 | $RbNa_3Li_8(Li(SiO_4))_4$ | 5.855e-1 | 5.761e-1 | 3.648e-1 | 2.216e-1 | 7.972 | -0.061 |
| 78326 | $Li_{10}(Si_2PbO_{10})$ | 5.724e+2 | 7.318e+2 | 1.398e+3 | 1.823e+3 | 1.453 | 0.283 |
| 78819 | $Li_{10}N_3Br$ | 3.298e+2 | 1.192e+3 | 2.010e+3 | 2.815e+3 | 2.597e-2 | 0.435 |
| 86184 | $LiZn(AsO_4)$ | 1.117e-1 | 1.390e-1 | 8.598e-2 | 2.360e-10 | 5.009e+26 | -2.436 |
| 86458 | $Li_3Sc_2(PO_4)_3$ | 2.132e+2 | 6.799e+2 | 5.602e+2 | 7.723e+2 | 7.987e-1 | 0.279 |
| 87596 | $Li_2(TiO)(SiO_4)$ | 4.022e-01 | 6.572e-10 | 5.476e-10 | 4.694e-10 | 1.072e+32 | -3.206 |
| 92708 | $Li(AlSiO_4)$ | 3.725e-3 | 3.332e-2 | 3.937e-2 | 3.443e-2 | 2.504e-7 | 0.455 |
| 95972 | $Li_2(MgSiO_4)$ | 6.694e-2 | 5.208e-1 | 6.012e-1 | 2.268e-1 | 1.255e-4 | 0.323 |
| 202115 | $NaLi_3(SiO_4)$ | 4.066e-1 | 9.919e-10 | 8.266e-10 | 7.085e-10 | 2.478e+31 | -3.142 |
| 202116 | $NaLi_3GeO_4$ | 1.426e-1 | 1.235e-1 | 3.641e-1 | 6.537e-10 | 6.402e+24 | -2.255 |
| 241234 | $Li_3Sc(BO_3)_2$ | 9.860e-10 | 3.113e-1 | 6.573e-10 | 3.655e+1 | 1.586e-35 | 2.586 |
| 252215 | $Li_3AlSiO_5$ | 4.912e-1 | 1.963e-1 | 7.578e-10 | 6.495e-10 | 1.655e+40 | -3.703 |

| | | | | | | | |
|---|---|---|---|---|---|---|---|
| 253895 | $Li_{10}Si_2P_6$ | 4.076 | 2.398 | 1.538e+1 | 7.410e+1 | 9.315e-06 | 0.549 |
| 257740 | $LiGa_{0.5}Al_{0.5}GeO_4$ | 4.407e-10 | 3.525e-10 | 2.938e-10 | 2.518e-10 | 1.175e-09 | 0.0 |
| 262642 | $In_2Li_2SiS_6$ | 7.233e-1 | 3.057 | 1.545e+2 | 5.927e+1 | 2.546e-10 | 0.934 |
| 262643 | $In_2Li_2GeS_6$ | 2.952e-10 | 7.809 | 2.034e+2 | 2.910e+2 | 2.814e-56 | 4.589 |
| 402341 | LiBeN | 3.459e-1 | 2.325e-1 | 8.006e-2 | 9.694e-2 | 3.598e+1 | -0.15 |
| 413355 | $(LiI)_2(Li_3(SbS_3))$ | 3.776e+2 | 1.049e+3 | 1.983e+3 | 2.650e+3 | 5.336e-2 | 0.408 |
| 424834 | $Li_3SbS_3$ | 8.335e-10 | 4.754e+2 | 1.546e+3 | 1.635e+3 | 4.350e-56 | 4.654 |
| 424835 | $Li_3AsS_3$ | 1.216e+3 | 1.468e+3 | 2.479e+3 | 3.150e+3 | 7.378 | 0.247 |
| 431367 | $Li_2SiP_2$ | 3.286e+2 | 6.504e+2 | 1.392e+3 | 2.373e+3 | 4.137e-2 | 0.408 |

Table S6. Oxide compounds that passed the threshold of activation barriers

| **ICSD-IDs** | **Compositions** | **Structure Type** | **Activation barrier** | **ESW** |
|---|---|---|---|---|
| 9987 | $Li_6Ga_2(BO_3)_4$ | $Li_3AlB_2O_6$ | 0.826 | 1.654 |
| 15631 | $Li_7(SbO_6)$ | | 0.228 | 1.137 |
| 23634 | $Li_{10}(Zn_4O_9)$ | | 0.627 | 1.405 |
| 26817 | $LiAl(Si_2O_6)$ | $LiAlSi_2O_6$ | 0.272 | 0 |
| 35250 | $K_2Li_{14}(Pb_3O_{14})$ | $K_2Li_{14}Pb_3O_4$ | 0.998 | 0.553 |
| 40245 | $Li_3BiO_3$ | | 0.573 | 0.977 |
| 40457 | $LiSbS_2$ | $AgAsS_2$ | 0.349 | 0.160 |
| 59381 | $Li_3(AsS_3)$ | | 0.260 | 0.203 |
| 59640 | $Li_4Zn(PO_4)_2$ | $Li_4O_8P_2Zn$ | 0.387 | 1.772 |
| 69967 | $NaLi_2(PO_4)$ | $Li_3PO_4$ | 0.429 | 3.190 |
| 71035 | $KLi_6(BiO_6)$ | $KLi_6IrO_6$ | 0.272 | 1.064 |
| 72840 | $Li_6K(BiO_6)$ | | 0.611 | 1.063 |
| 74864 | $CsKNa_2Li_8(Li(SiO_4))_4$ | $CsKNa_2Li_8(LiSiO_4)_4$ | 0.297 | 2.382 |
| 78326 | $Li_{10}(Si_2PbO_{10})$ | | 0.283 | 0 |
| 78819 | $Li_{10}N_3Br$ | | 0.435 | 0.53 |
| 86458 | $Li_3Sc_2(PO_4)_3$ | $Li_3Fe_2(PO_4)_3$ | 0.279 | 0 |
| 92708 | $Li(AlSiO_4)$ | $LiGaSiO_4$ | 0.455 | 2.667 |
| 95972 | $Li_2(MgSiO_4)$ | $Li_2ZnSiO_4$ | 0.323 | 2.739 |
| 253895 | $Li_{10}Si_2P_6$ | | 0.549 | 0.373 |
| 262642 | $In_2Li_2SiS_6$ | $Cd_4GeS_6$ | 0.934 | 0.755 |
| 413355 | $(LiI)_2(Li_3(SbS_3))$ | | 0.408 | 0.325 |
| 424835 | $Li_3AsS_3$ | | 0.247 | 0.204 |
| 431367 | $Li_2SiP_2$ | | 0.408 | 0.427 |

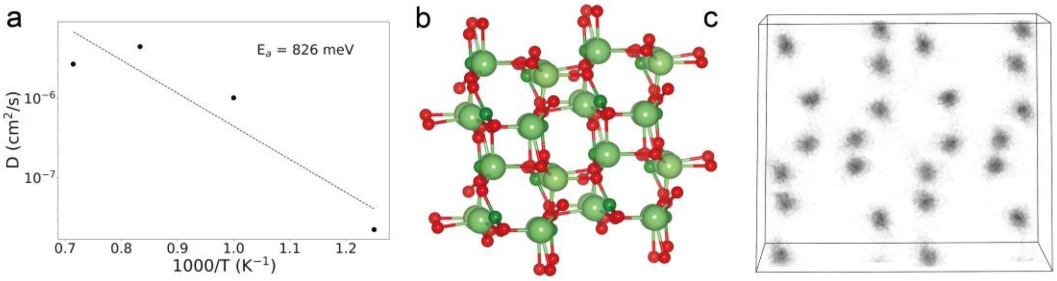


Figure S1. AIMD simulations of $Li_6Ga_2(BO_3)_4$. a) Arrhenius plot of lithium-ion diffusion coefficient. b) The structure schematic. c) Isosurface of lithium-ion probability density from the 800-1400K AIMD simulation.

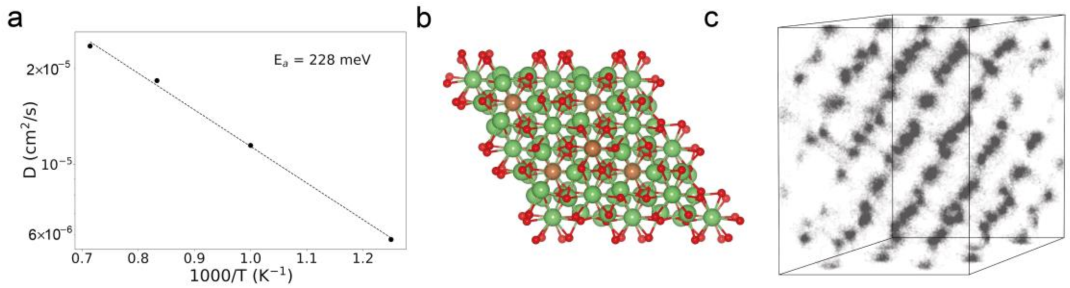


Figure S2. AIMD simulations of $Li_7SbO_6$. a) Arrhenius plot of lithium-ion diffusion coefficient. b) The structure schematic. c) Isosurface of lithium-ion probability density from the 800-1400K AIMD simulation.

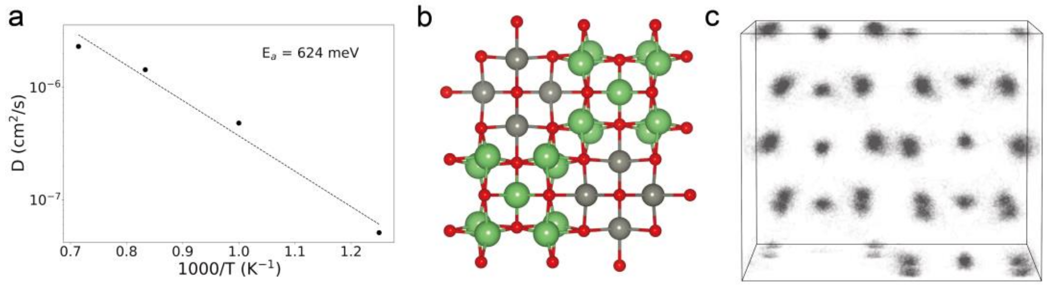


Figure S3. AIMD simulations of $Li_{10}Zn_4O_9$. a) Arrhenius plot of lithium-ion diffusion coefficient. b) The structure schematic. c) Isosurface of lithium-ion probability density from the 800-1400K AIMD simulation.

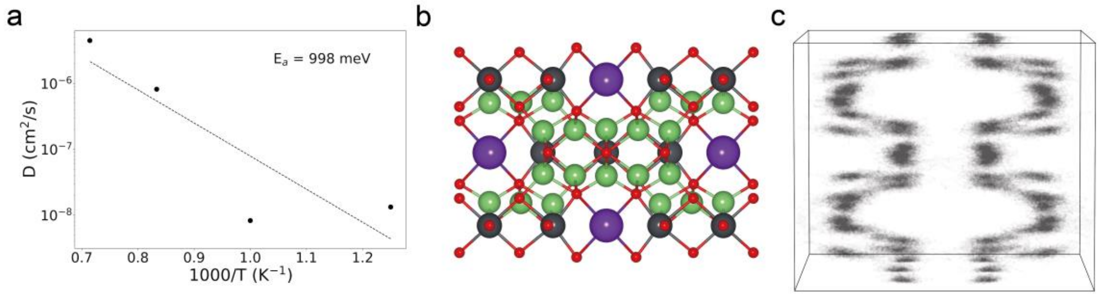


Figure S4. AIMD simulations of $K_2Li_{14}Pb_3O_{14}$. a) Arrhenius plot of lithium-ion diffusion coefficient. b) The structure schematic. c) Isosurface of lithium-ion probability density from the 800-1400K AIMD simulation.

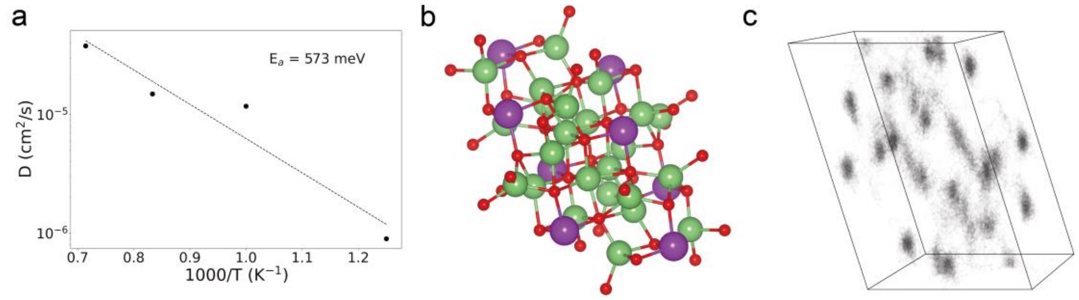


Figure S5. AIMD simulations of $Li_3BiO_3$. a) Arrhenius plot of lithium-ion diffusion coefficient. b) The structure schematic. c) Isosurface of lithium-ion probability density from the 800-1400K AIMD simulation.

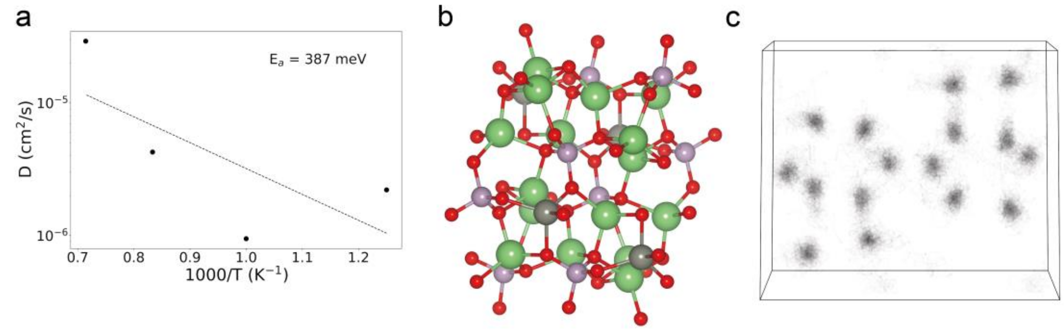


Figure S6. AIMD simulations of $Li_4Zn(PO_4)_2$. a) Arrhenius plot of lithium-ion diffusion coefficient. b) The structure schematic. c) Isosurface of lithium-ion probability density from the 800-1400K AIMD simulation.

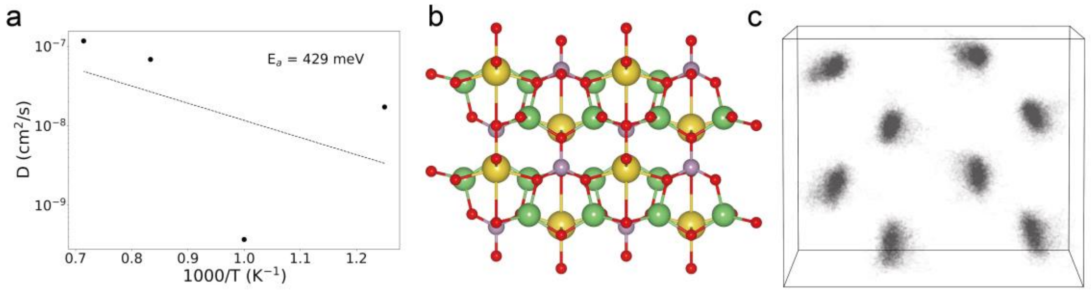


Figure S7. AIMD simulations of $NaLi_2PO_4$. a) Arrhenius plot of lithium-ion diffusion coefficient. b) The structure schematic. c) Isosurface of lithium-ion probability density from the 800-1400K AIMD simulation.

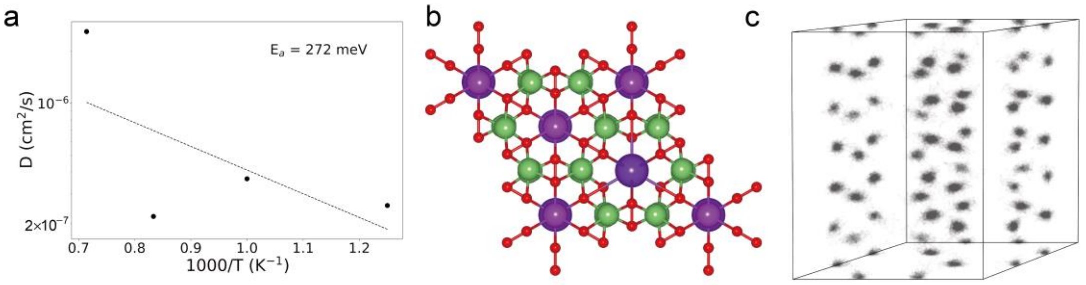


Figure S8. AIMD simulations of $KLi_6BiO_6$. a) Arrhenius plot of lithium-ion diffusion coefficient. b) The structure schematic. c) Isosurface of lithium-ion probability density from the 800-1400K AIMD simulation.

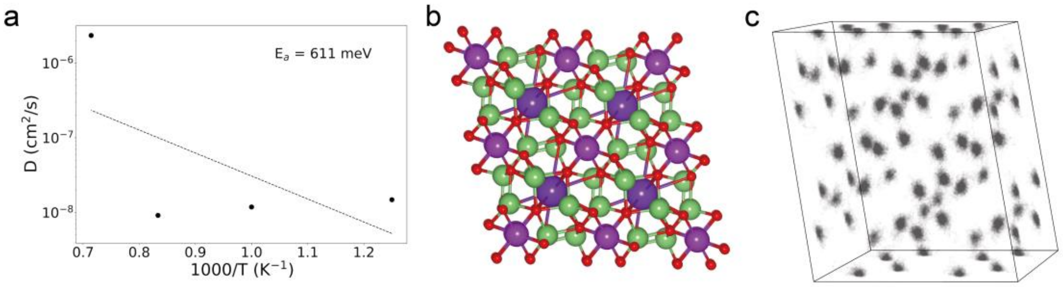


Figure S9. AIMD simulations of $Li_6KBiO_6$. a) Arrhenius plot of lithium-ion diffusion coefficient. b) The structure schematic. c) Isosurface of lithium-ion probability density from the 800-1400K AIMD simulation.

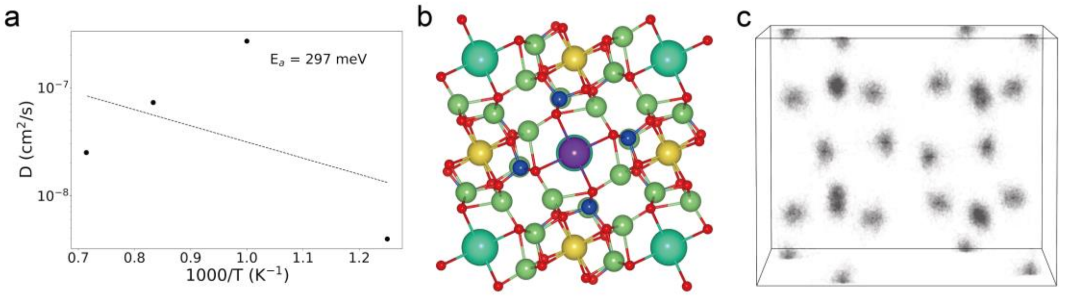


Figure S10. AIMD simulations of $CsKNa_2Li_8(Li(SiO_4))_4$. a) Arrhenius plot of lithium-ion diffusion coefficient. b) The structure schematic. c) Isosurface of lithium-ion probability density from the 800-1400K AIMD simulation.

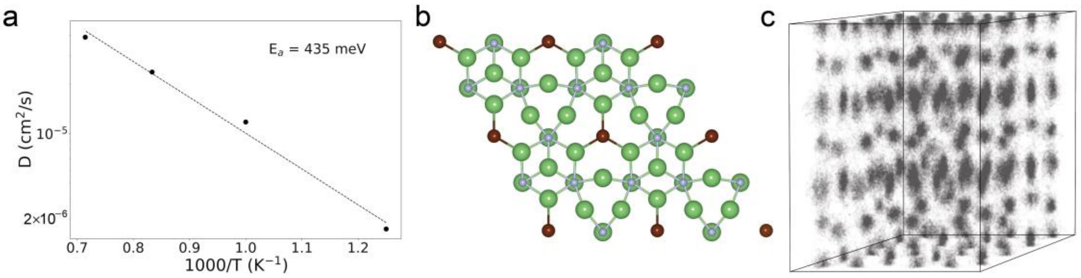


Figure S11. AIMD simulations of $Li_{10}N_3Br$. a) Arrhenius plot of lithium-ion diffusion coefficient. b) The structure schematic. c) Isosurface of lithium-ion probability density from the 800-1400K AIMD simulation.

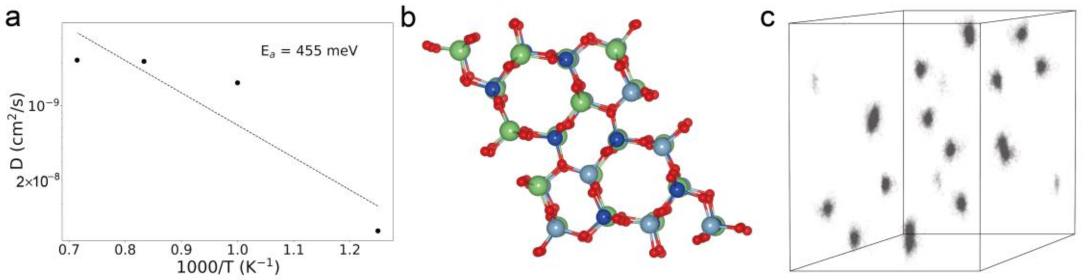


Figure S12. AIMD simulations of $LiAlSiO_4$. a) Arrhenius plot of lithium-ion diffusion coefficient. b) The structure schematic. c) Isosurface of lithium-ion probability density from the 800-1400K AIMD simulation.

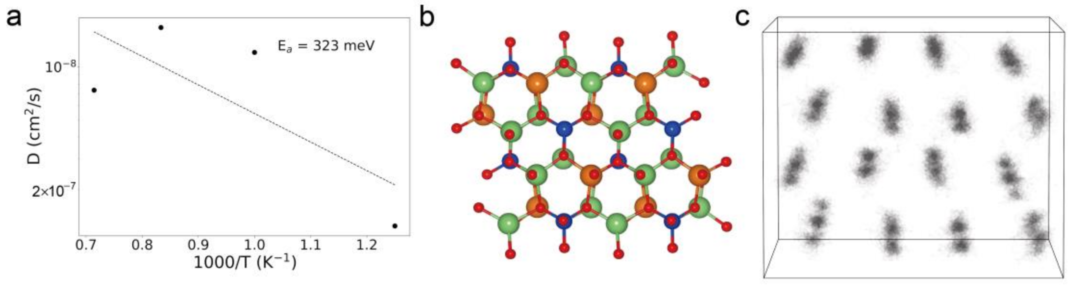


Figure S13. AIMD simulations of $Li_2MgSiO_4$. a) Arrhenius plot of lithium-ion diffusion coefficient. b) The structure schematic. c) Isosurface of lithium-ion probability density from the 800-1400K AIMD simulation.

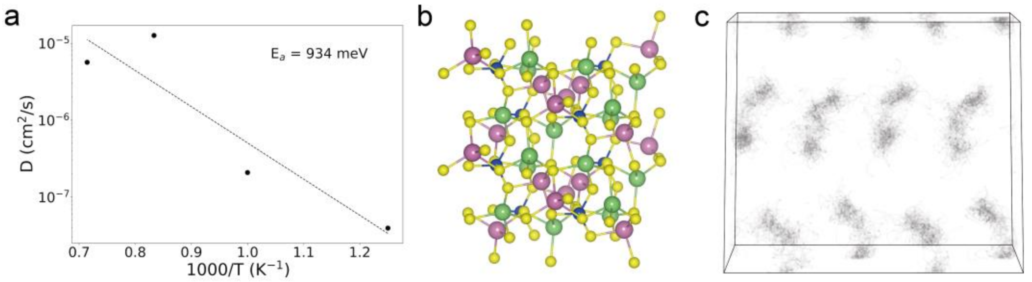


Figure S14. AIMD simulations of $In_2Li_2SiS_6$. a) Arrhenius plot of lithium-ion diffusion coefficient. b) The structure schematic. c) Isosurface of lithium-ion probability density from the 800-1400K AIMD simulation.
